# Supplementary material for: MarsRL: Advancing Multi-Agent Reasoning System via Reinforcement Learning with Agentic Pipeline Parallelism
Source: arXiv:2511.11373 source file (2025-11-14)
Supplement: Supplementary file 1 [file appendix.tex]

\section{Appendix}
\label{sec:appendix}
Figure \ref{fig:apdx_figure1} present the full result of  Leaderboard of LMSYS Chatbot Arena by May 18, 2025.
\begin{figure}[!htb]
\centering
     \includegraphics[width=0.8\textwidth, scale=1, trim=0 175 0 0 ,clip]{figures/Leaderboard.png}
     \caption{Full Leaderboard of LMSYS Chatbot Arena by May 18, 2025.}
     \label{fig:apdx_figure1}
\end{figure}
